# Supplementary material for: Ev-TTA: Test-Time Adaptation for Event-Based Object Recognition
Source: arXiv:2203.12247 source file (2022-03-28)
Supplement: Supplementary file 1 [file sim2real.tex]

\begin{table}[]
\centering
\resizebox{1.0\columnwidth}{!}{%
\begin{tabularx}{1.15\columnwidth}{l|c|c|c|c}
\toprule
Representation & Sim & None & Tent~\cite{tent} & Ev-TTA\\ \midrule
Timestamp Image~\cite{timestamp_image} & 53.53 & 31.36 & 38.96 & \textbf{40.66}\\ 
Binary Event Image~\cite{binary_image_2} & 54.63 & 26.62 & 38.67 & \textbf{40.94}\\ 
Event Histogram~\cite{event_driving} & 44.44 & 21.97 & 30.2 & \textbf{34.87}\\ \bottomrule
\end{tabularx}
}
\caption{Evaluation results on Sim2Real gap.}
\label{tab:supp_sim2real}
\end{table}
